# Supplementary material for: Learning Color Compatibility in Fashion Outfits
Source: arXiv:2007.02388 source file (2020-07-05)
Supplement: Supplementary file 1 [file supp.tex]

\clearpage
\begin{center}
\Large \textbf{Supplementary Material: Learning Color Compatibility in Fashion Outfits}
\end{center}

\begin{appendix}
\section{Design Choices for Proposed Joint Training Scheme}
In this section, we would like to further clarify several design choices we have made for the proposed joint training of compatibility prediction and outfit clustering.

\subsection{Interpreting Compatibility from Outfit Clusters}
In our work, we propose a new method to interpret compatibility prediction. As introduced in Section \ref{subsec:fashion_compatibility}, some recent work also tended to interpreting their compatibility models via disentanglement \cite{[2018ICMR]Interpretable,[2019arxiv]Toward,[2019SIGIR]Interpretable,[2019ICCV]Learning}. Nevertheless, these studies only disentangled the item representations. In \cite{[2018ICMR]Interpretable,[2019arxiv]Toward,[2019SIGIR]Interpretable}, the item representations are divided according to their attributes such as categories, shapes, textures, etc. Tan \cite{[2019ICCV]Learning} proposed to learn multiple masks of item embeddings such that each mask focuses on one item attribute. However, it is difficult to interpret the compatibility of entire outfits from such embedding disentanglement of individual items. To address such difficulty, we propose to interpret outfit compatibility at the outfit level. This is achieved by obtaining disentanglement on the outfit embeddings rather than the item embeddings. 
To obtain the disentanglement that is meaningful for interpreting compatibility predictions, we propose to automatically cluster the corresponding embeddings, whereas the disentanglement in \cite{[2018ICMR]Interpretable,[2019arxiv]Toward,[2019SIGIR]Interpretable} was manually performed on attributes, and may not be meaningful for interpreting the compatibilities. 
%In \cite{[2019ICCV]Learning}, learnable masks were used to select useful parts of item embeddings. Since such masks are not guaranteed to have disentanglement, extra $l_1$ regularization was used to encourage disentanglement. In our work, we propose to use clustering instead of masks for its intrinsic property of disentanglement.

\subsection{Pseudo Label Assignment}
As introduced in Section \ref{subsec:joint}, we generate pseudo labels by fusing the ground-truth compatibility labels and the cluster assignments. We first cluster the outfits without any supervision from the compatibility labels. Then based on the compatibility labels, we divide the clusters into two meta-groups, positive and negative. We perform a compatibility check on each sample to make sure it shares the same compatibility label as the cluster it belongs to. If a sample has a different compatibility label to its initially assigned cluster, we will assign this sample to the nearest cluster that shares the same compatibility label.

For the positive samples, multiple clusters are used to help us understand different modes of fashion compatibility. For the negative samples, on the other hand, there is little interest to further partition them. 
%We also compared the results with multiple negative clusters and did not observe any improvement.
Therefore we only assign one negative cluster for computational efficiency. 

In Figure \ref{fig:TSNE}, we visualize outfit embeddings on the validation set of Polyvore Outfits with one negative cluster and three positive clusters. Different colors indicate the predictions made by our model. The samples with wrongly predicted compatibility are denoted in black color. The other colors indicate predicted clusters of the samples whose compatibilities are correctly predicted. It shows that the embeddings of negative samples are concentrated after the joint training. Thus there is no need to further divide the negative samples. The experimental results also verified that assigning multiple negative clusters does not improve the performance. 
\begin{figure}
\centering
\includegraphics[trim=50 40 50 40, clip,width=\linewidth]{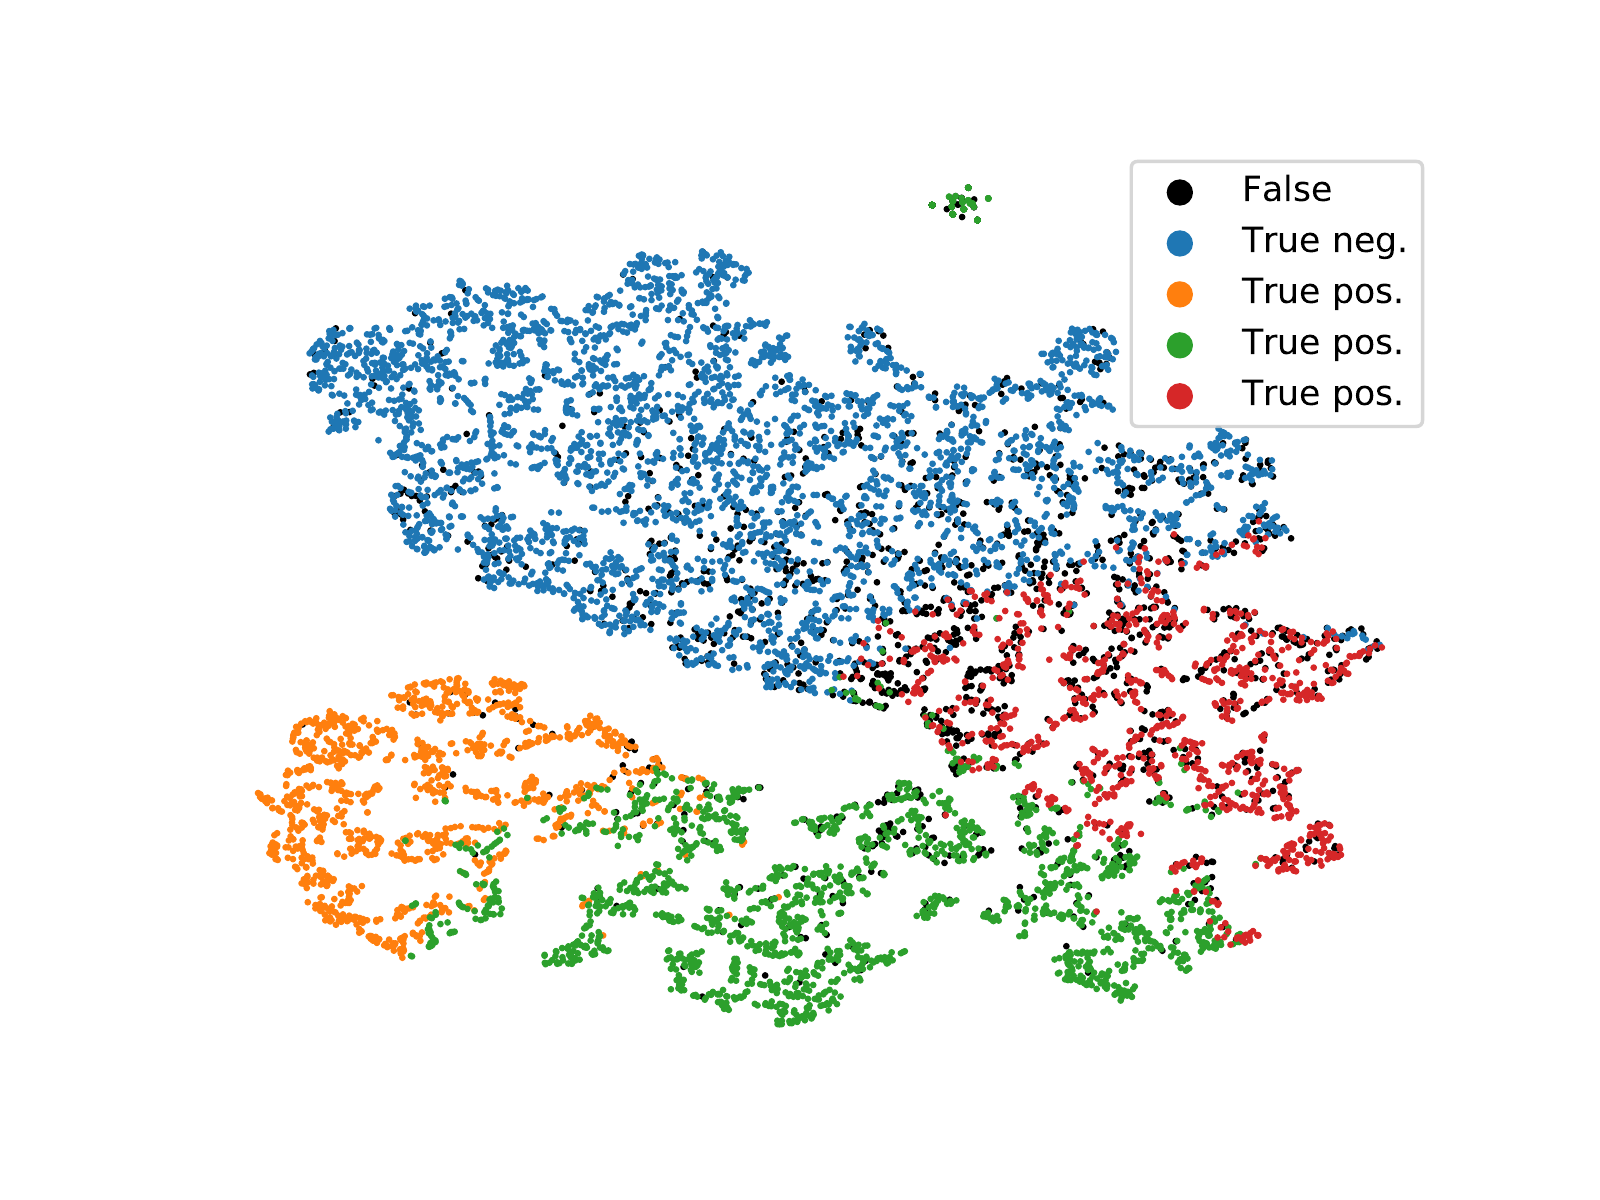}
\caption{TSNE visualization of the outfit embeddings obtained from a model trained with one negative cluster. The black points are the samples whose compatibility are wrongly predicted and the points in other colors are the samples whose compatibility are correctly predicted. Furthermore, each color indicates a different cluster predicted by the trained model.}
\label{fig:TSNE}
\end{figure}

\subsection{Global and Local Supervision}
\begin{figure}
\centering
\includegraphics[trim=0 0 520 0, clip,width=\linewidth]{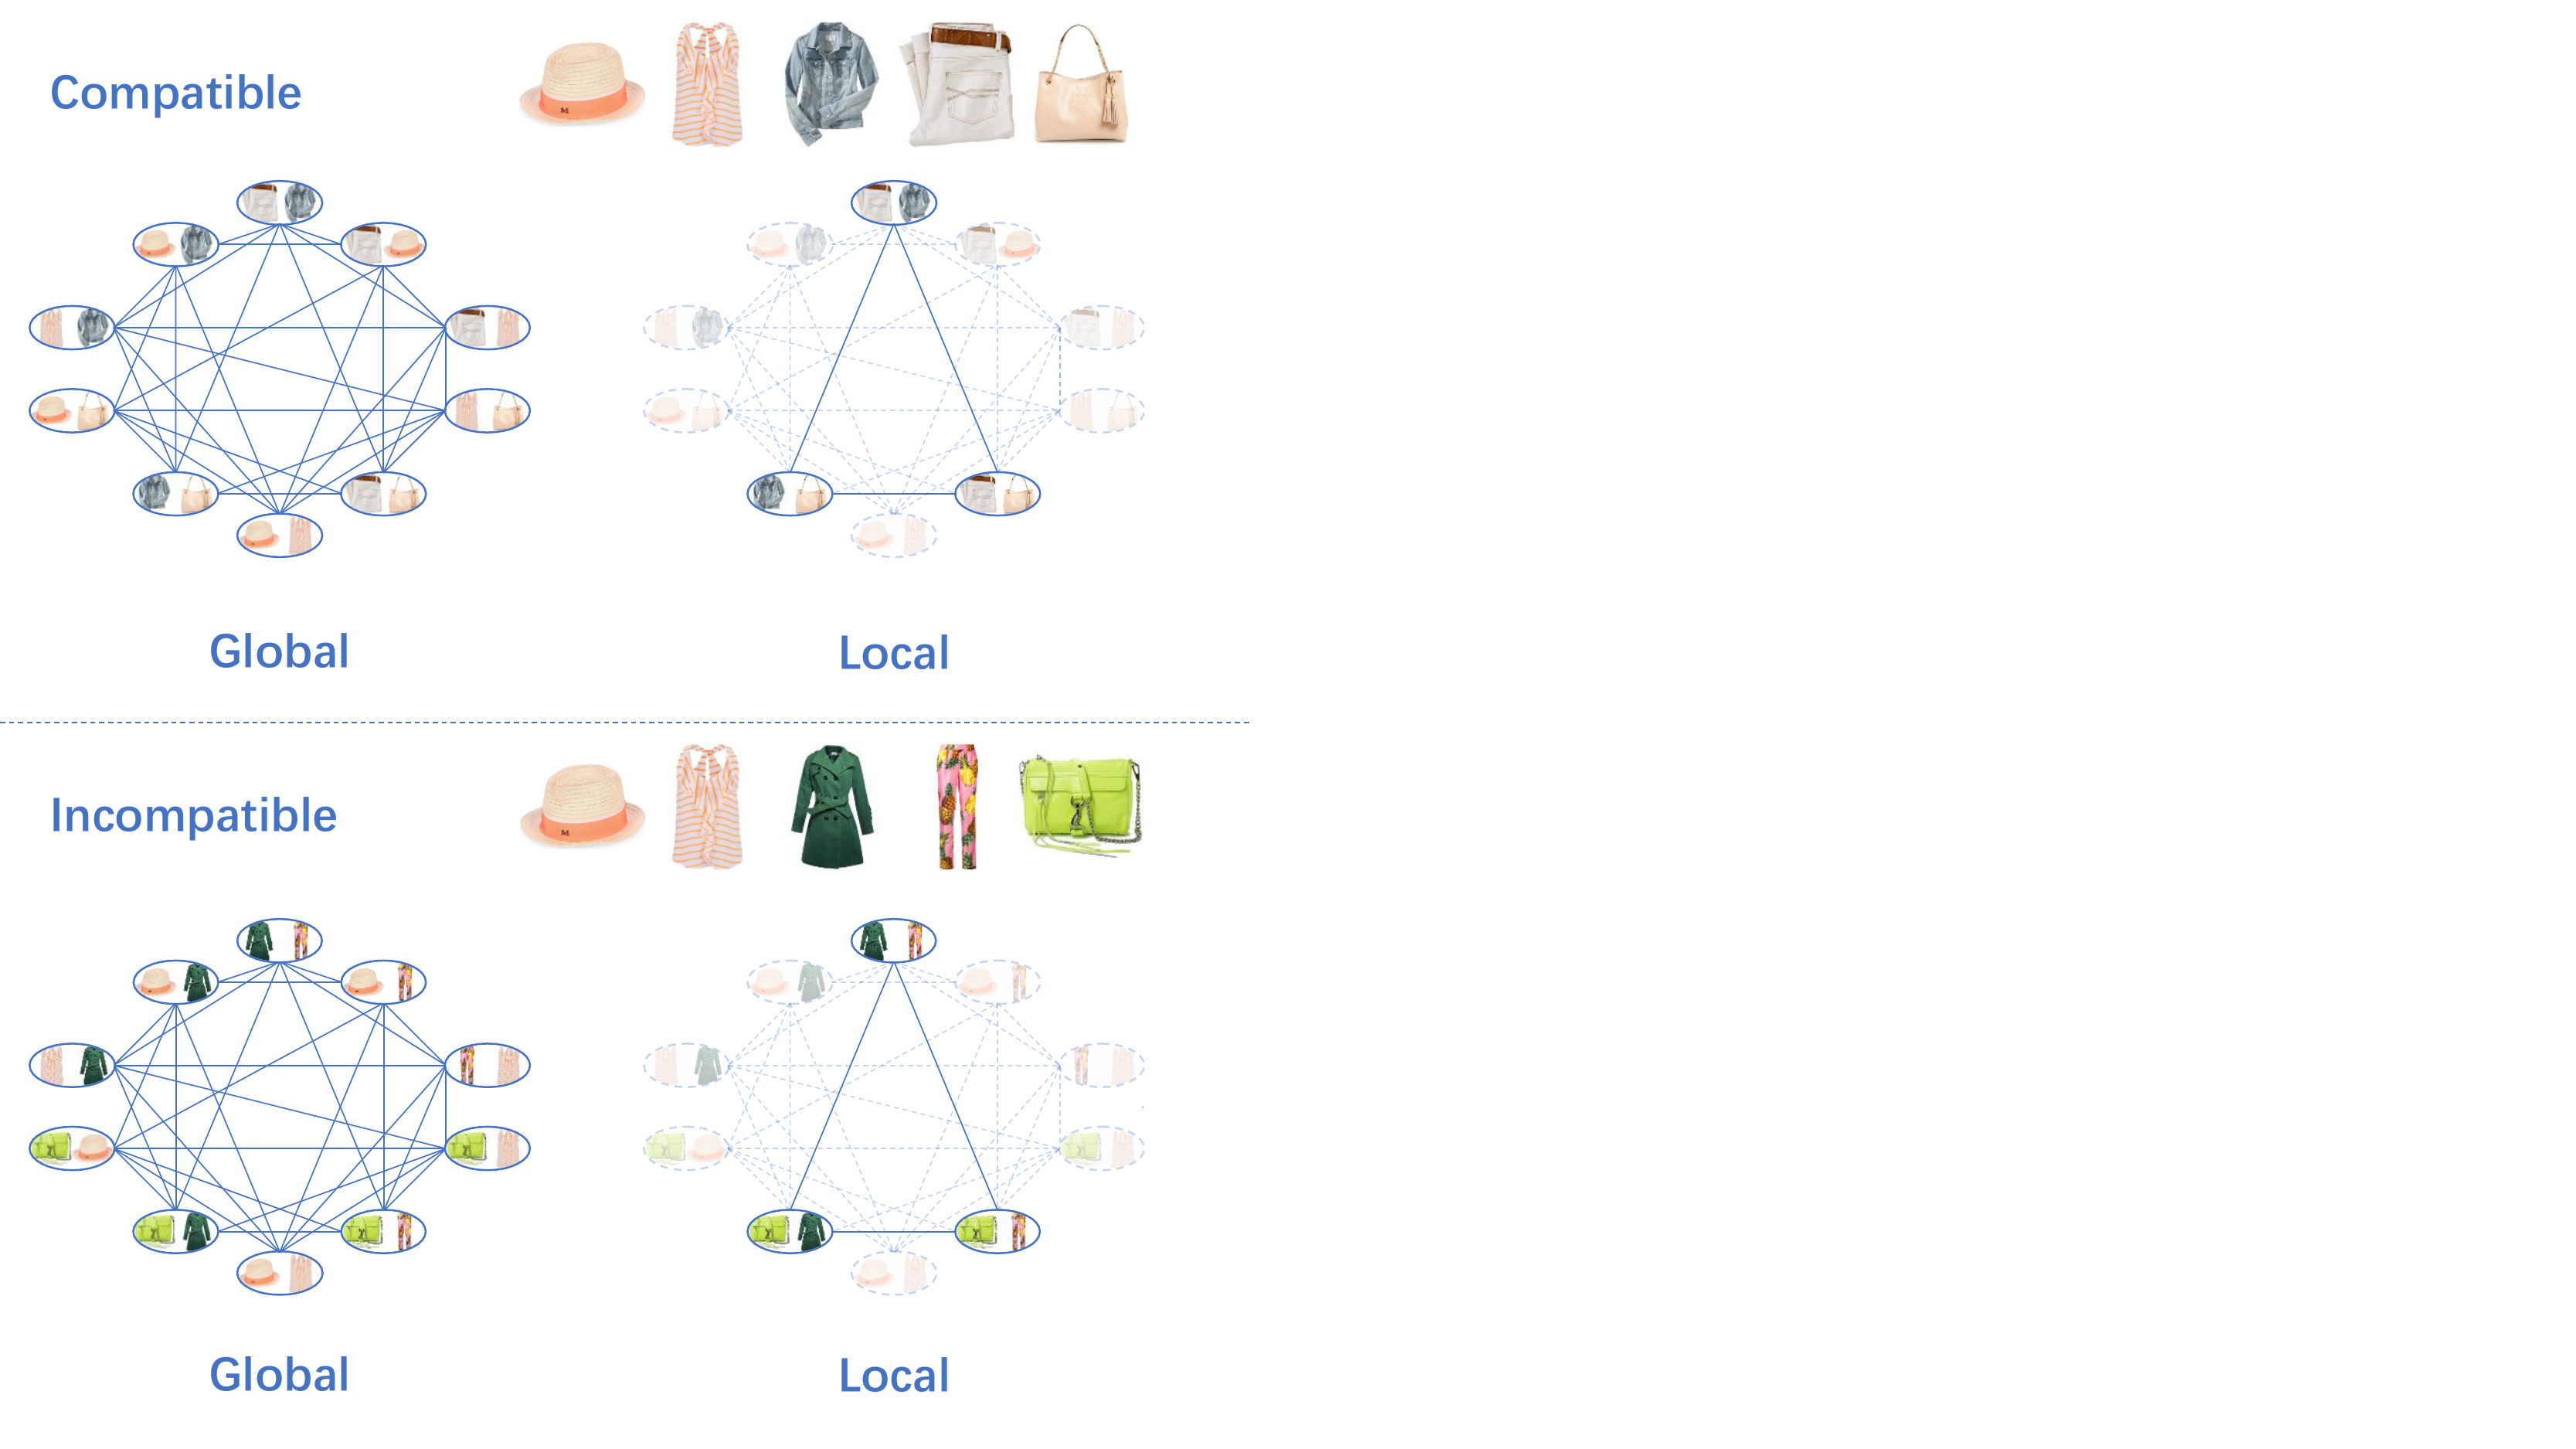}
\caption{Graph constructions for global and local supervision of a given pair of samples. For global supervision, all items in the outfits are used. For local supervision, common items in the positive-negative sample pair are not used. Eliminated nodes and edges are denoted in dotted lines.}
\label{fig:global_local}
\end{figure}
The original data collected in Polyvore Outfits \cite{[2018ECCV]Learning} and Maryland Polyvore \cite{[2017MM]Learning} only contains compatible outfits as positive samples. For the tasks of compatibility prediction and fill-in-the-blank, negative outfits were constructed by randomly sampling items in the data. We also follow this random sampling strategy to construct negative samples for our training procedure. For each positive-negative pair of samples, the negative sample was generated by randomly replacing some of the items.

We propose to use the two loss functions in Equations \ref{eq:l1} and \ref{eq:l2}. Figure \ref{fig:global_local} illustrates the corresponding graph construction where each sample contains five items and the two samples have two items in common.

The first loss introduced in Equation \ref{eq:l1} is a global loss that is applied to each sample pair entirely. As illustrated in Figure \ref{fig:global_local}, the compatible outfit on the top represents a positive input $\mathbf{x}_{i,pos}$ and the incompatible outfit at the bottom represents a negative input $\mathbf{x}_{i,neg}$. We construct the graphs using every items provided in the sample pair, as illustrated in Figure \ref{fig:global_local} on the left. Using the method described in Section \ref{subsec:joint} we obtain the multi-class pseudo labels $\tilde{y}_{i,pos}$ and $\tilde{y}_{i,neg}\in \{0,1,\cdots,C-1\}$ for the positive and negative samples, respectively. Let $g(\cdot)$ denotes the softmax output vector predicted by the proposed system and $[\cdot]_c$ denotes the $c$th element, the global loss can be formulated as

\begin{equation}
\begin{split}
l_1 = \sum_i \left[-\log\left( [g(\mathbf{x}_{i,pos})]_{\tilde{y}_{i,pos}}\right) - \log\left([g(\mathbf{x}_{i,neg})]_{\tilde{y}_{i,neg}} \right) \right].
\end{split}
\end{equation}

The local supervision uses the second loss provided in Equation \ref{eq:l2}. It is only applied to some items in the given pairs. The correspondingly constructed graphs are shown on the right side of Figure \ref{fig:global_local}. Common items in the pair are ignored. Since the obtained outfit subsets may not follow the patterns in any clusters, we only use the binary compatibility labels for local supervision. Let $p(\cdot)$ denotes the sum of $[g(\cdot)]_c$ for all positive clusters $c$, i.e. the predicted probability that a sample is compatible, the local loss can be formulated as

\begin{equation}
\begin{split}
l_2 = \sum_i \left[ -\log \left( p(\hat{\mathbf{x}}_{i,pos}) \right) - \log \left( 1- p(\hat{\mathbf{x}}_{i,neg}) \right) \right].
\end{split}
\end{equation}

\subsection{Hyper-parameters}
We studied the effect of different choices of hyper-parameters and the results are listed in Tables \ref{tb:cluster} and \ref{tb:lambda}. The experiments are conducted on the validation set of Polyvore Outfits with color palettes. For each hyper-parameter, we varied its value while keeping other hyper-parameters unchanged.

\begin{table}
\begin{center}
\begin{tabular}{|l|c|c|}
\hline
\#clusters & 
Compat AUC & FITB Acc\\
\hhline{|=|=|=|}
3 & 0.84 & 54.2\\ 
5 & 0.84 & 58.8 \\
7 & 0.84 & 56.9 \\
9 & 0.84 & 55.1\\
\hline
\end{tabular}
\end{center}
\caption{Effect of different choices of cluster numbers. The experiments are conducted on the validation set of Polyvore Outfits with color palettes as fashion representations.}
\label{tb:cluster}
\end{table}

\begin{table}
\begin{center}
\begin{tabular}{|l|c|c|}
\hline
$\lambda$ & 
Compat AUC & FITB Acc\\
\hhline{|=|=|=|}
0 & 0.84 & 54.7\\ 
0.5 & 0.84 & 58.8 \\
1 & 0.84 &  57.1\\
5 & 0.83 & 50.5\\
\hline
\end{tabular}
\end{center}
\caption{Effect of different choices of $\lambda$. The experiments are conducted on the validation set of Polyvore Outfits with color palettes as fashion representations.}
\label{tb:lambda}
\end{table}

In general, we observe that the values of the number of clusters and the $\lambda$ in Equation \ref{eq:loss} mainly affect the FITB accuracy. Because the compatibility prediction task only requires binary predictions of the outfit compatibility, whereas the fill-in-the-blank task requires more insights of the outfit compatibility. From the ablation study in Section \ref{subsec:ablation}, we observe that the improvement of compatibility prediction mainly comes from our proposed graph construction.

An appropriate number of cluster helps the model better learn different compatible patterns. From experiments we find five clusters are appropriate for outfit clustering with color palettes as inputs.

The value of $\lambda$ determines the ratio between two loss functions in Equations \ref{eq:l1} and \ref{eq:l2}. The results show that a small value of $\lambda$ such as 0.5 or 1 will improve the FITB accuracy, as the auxiliary local supervision help the model learn subtle differences. A large value of $\lambda$ may hurt the performance, as the local supervision does not provide a global view and may not be accurate.

%%%%%%%%%%%%%%%%%%%%%%%%%%%%%%%
\section{Visualization Results}
\begin{figure*}
\centering
\includegraphics[trim=0 270 200 0, clip,width=\linewidth]{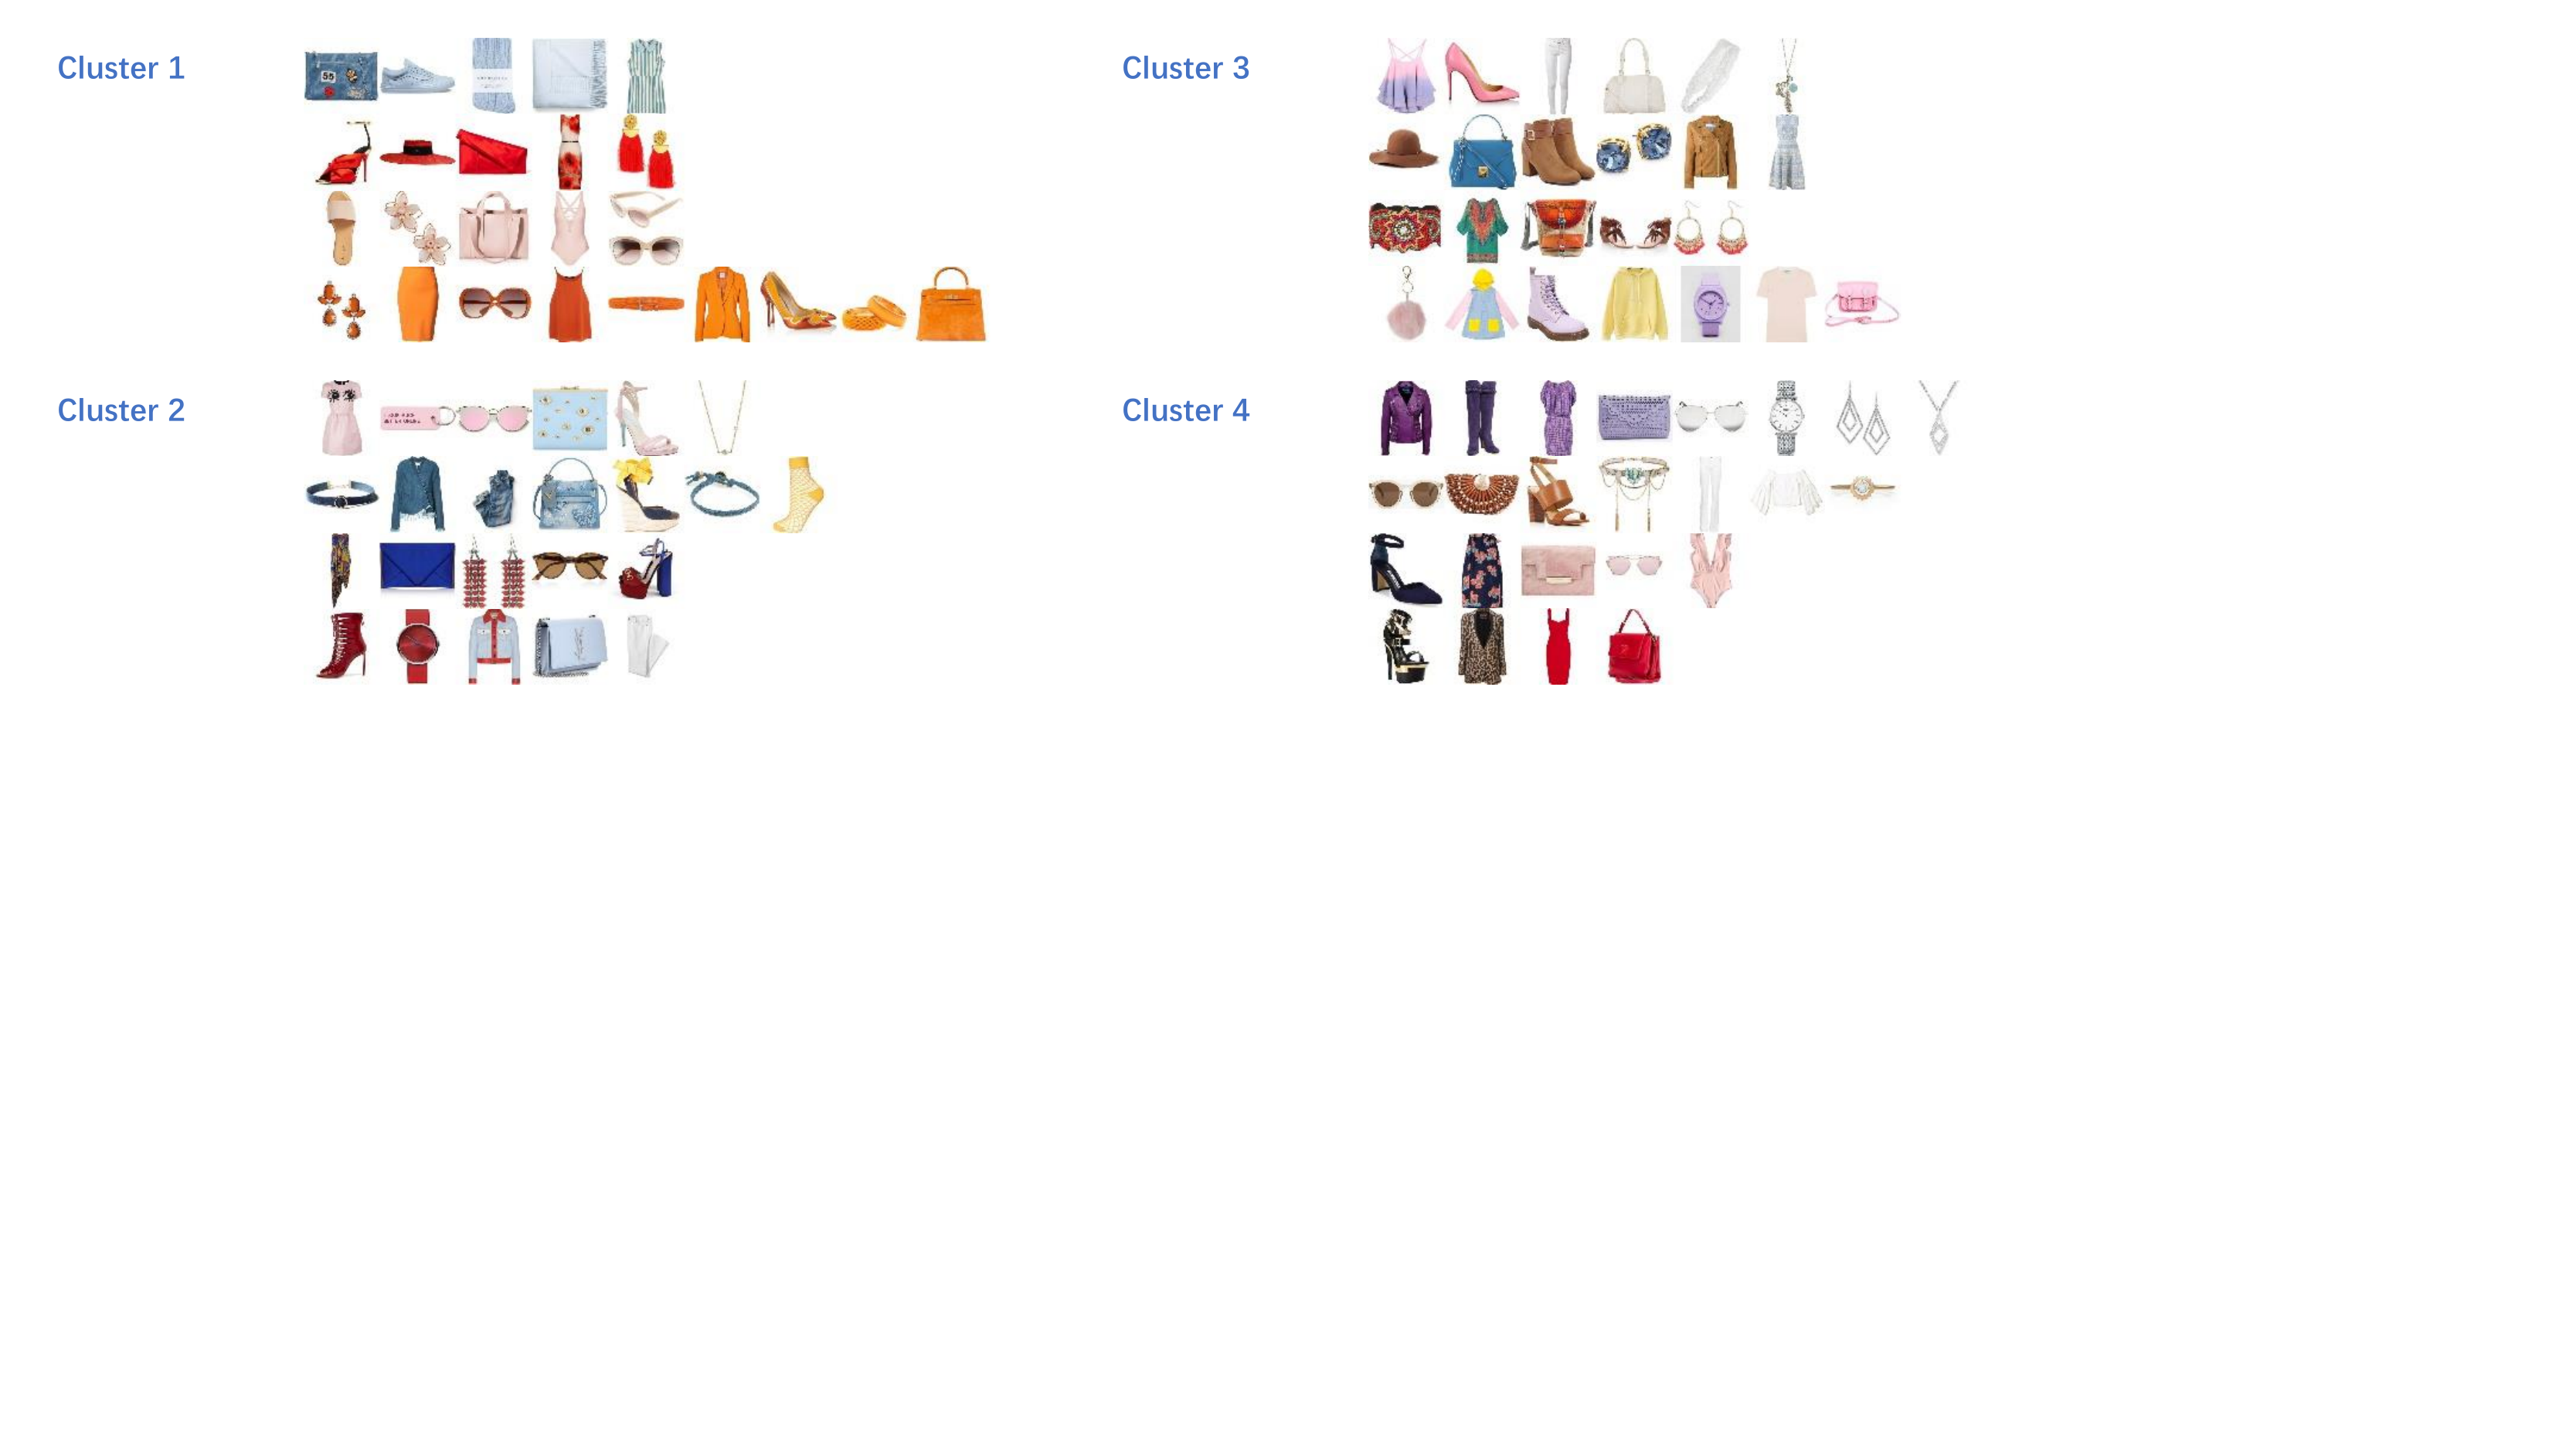}
\caption{Examples of outfits in each predicted cluster. The experiments were conducted on the testing set of the Polyvore Outfits dataset using the proposed method with color palettes. Each outfit is displayed in a row.}
\label{fig:supp_cluster}
\end{figure*}

In this section, we further show some visual examples of results obtained by the proposed method.

In Figure \ref{fig:supp_cluster}, outfit examples of each predicted cluster are shown. The experiments were conducted on the testing set of the Polyvore Outfit dataset using the proposed method with color palettes.

Unlike the cluster predicted using deep image features in Figure \ref{fig:sample_it} that reveals a color pattern, we show two other clusters in Figure \ref{fig:supp_sample_it}. They are also obtained by using deep image features and show mixed color patterns within each cluster, making it harder to interpret. 

\begin{figure*}
\begin{center}
\begin{subfigure}[b]{\linewidth}
	\centering
	\includegraphics[trim=0 0 0 0, clip,width=\linewidth]{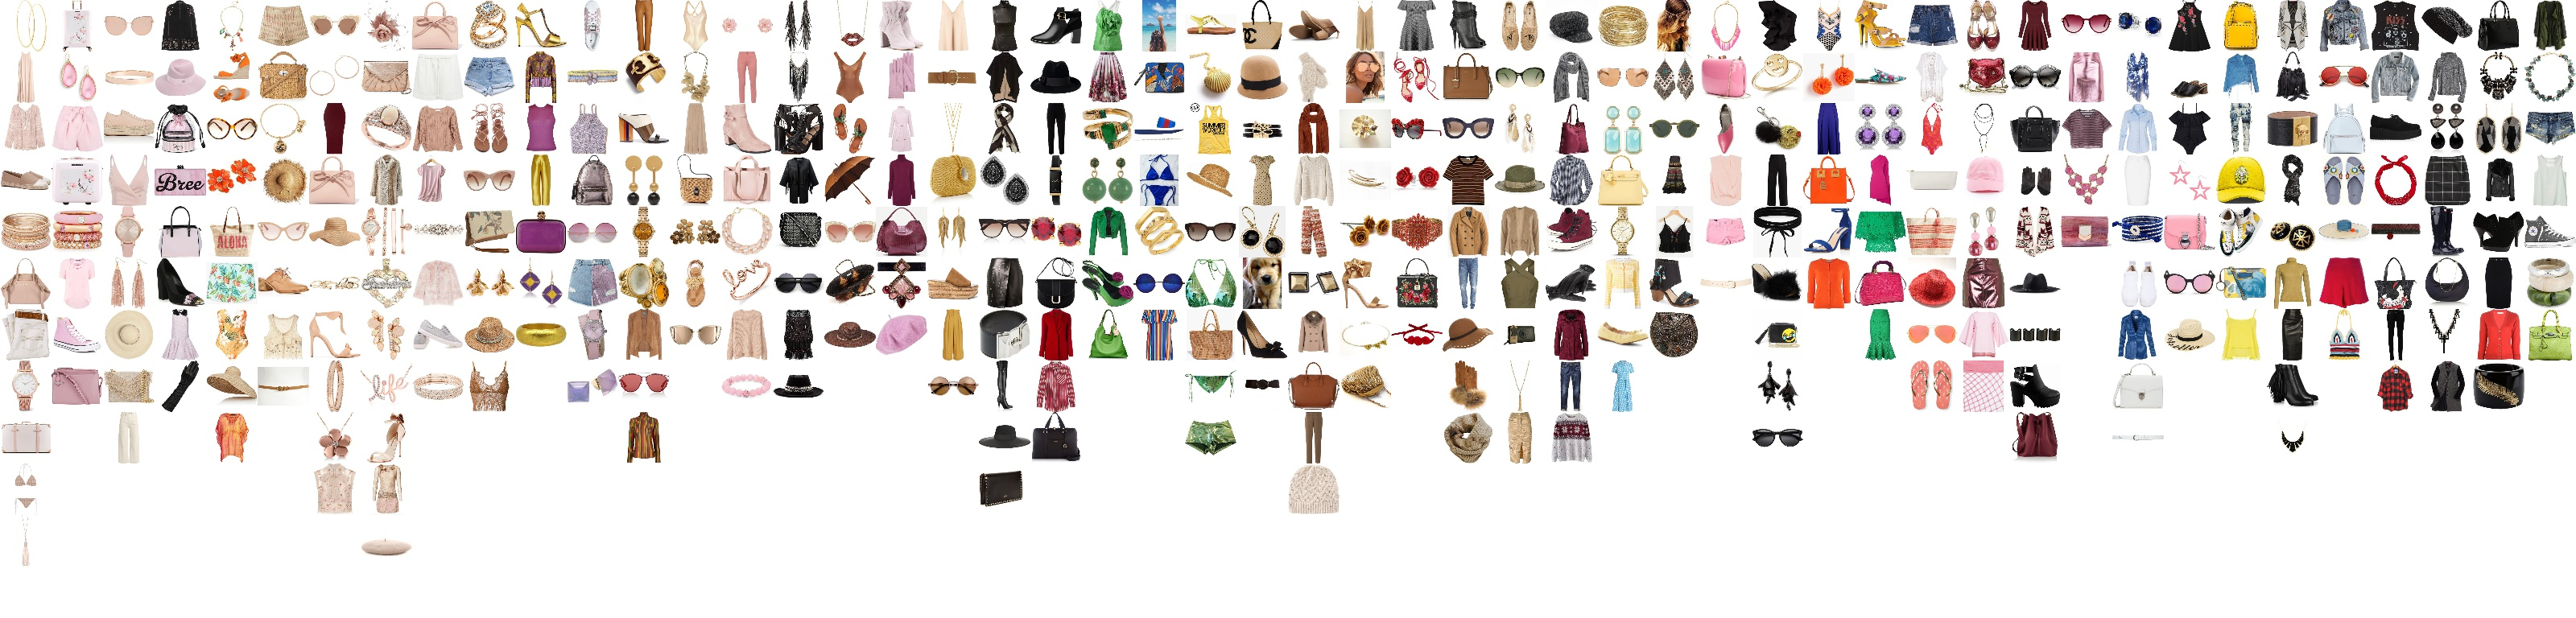}
	\caption{This cluster reveals two mixed color patterns. One pattern consists of similar colors, whereas the other pattern shows contrast colors.}
	\label{fig:supp_sample_it1}
\end{subfigure}
\begin{subfigure}[b]{\linewidth}
	\centering
	\includegraphics[trim=0 0 0 0, clip,width=\linewidth]{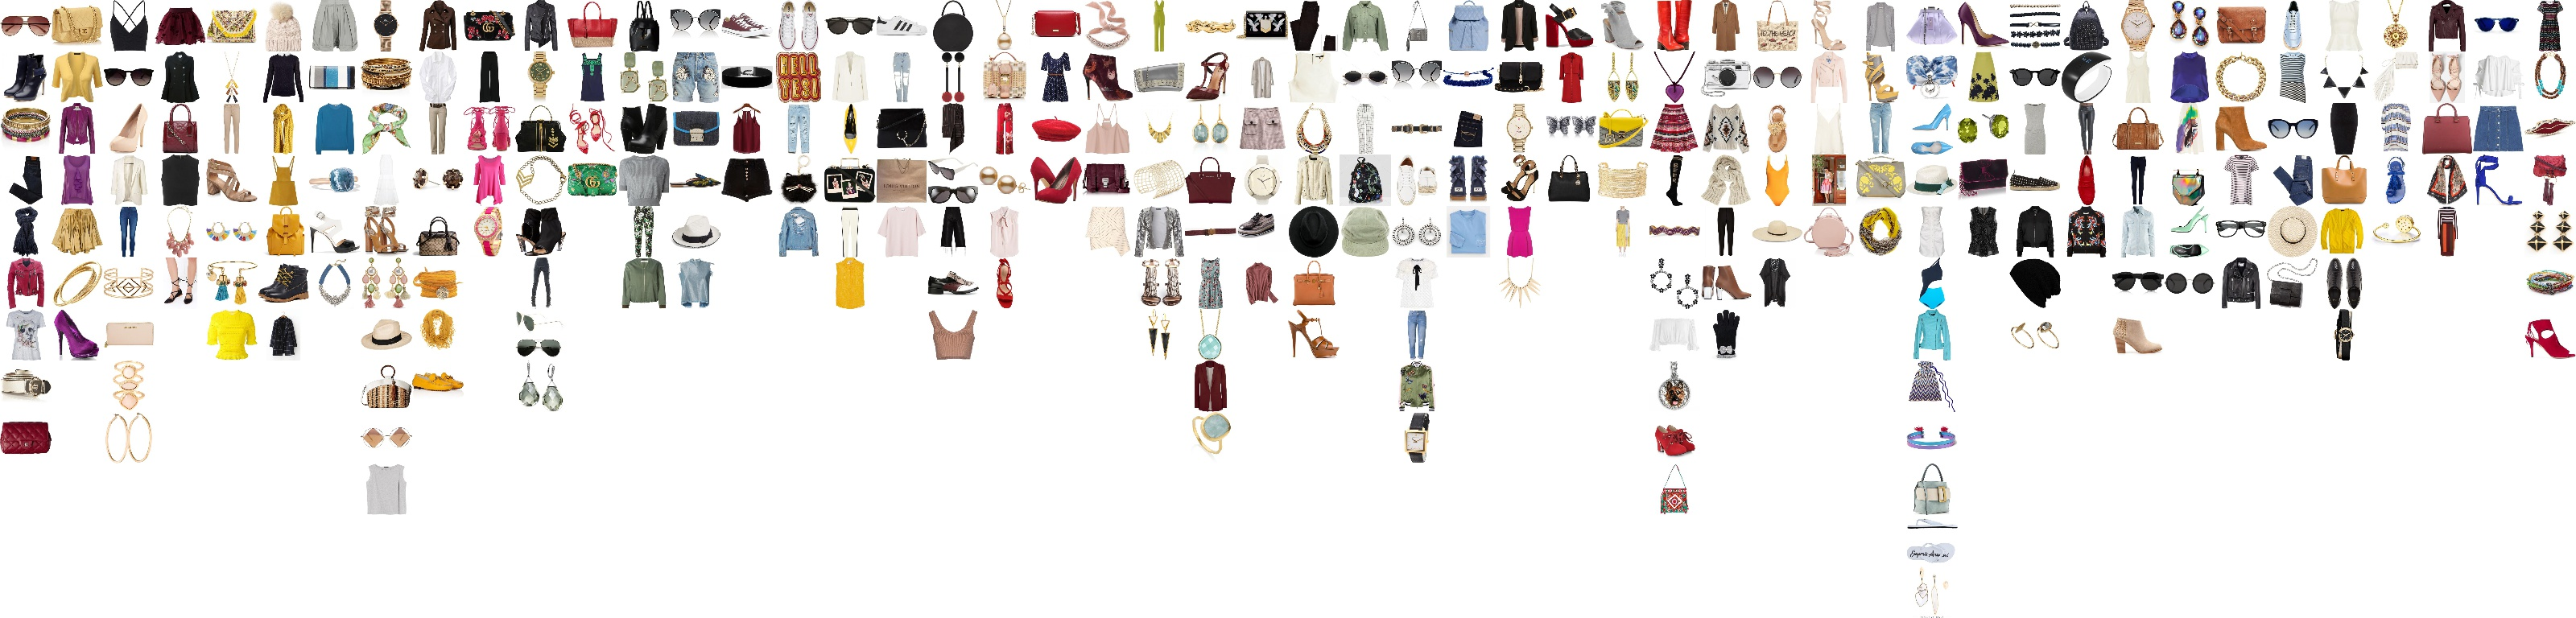}
	\caption{This cluster contains multiple color patterns that are hard to interpret directly.}
	\label{fig:supp_sample_it2}
\end{subfigure}
\end{center}
   \caption{Compatible outfit clusters predicted using color palettes as fashion representation. Due to limited space, we only display 50 outfits per cluster. The 50 outfits are shown on the left where items in the same column belong to the same outfit.}
\label{fig:supp_sample_it}
\end{figure*}

\end{appendix}
