# Supplementary material for: Learning Color Compatibility in Fashion Outfits
Source: arXiv:2007.02388 source file (2020-07-05)
Supplement: Supplementary file 2 [file figure_supp_cluster.tex]

\begin{figure*}
\centering
\includegraphics[trim=0 270 200 0, clip,width=\linewidth]{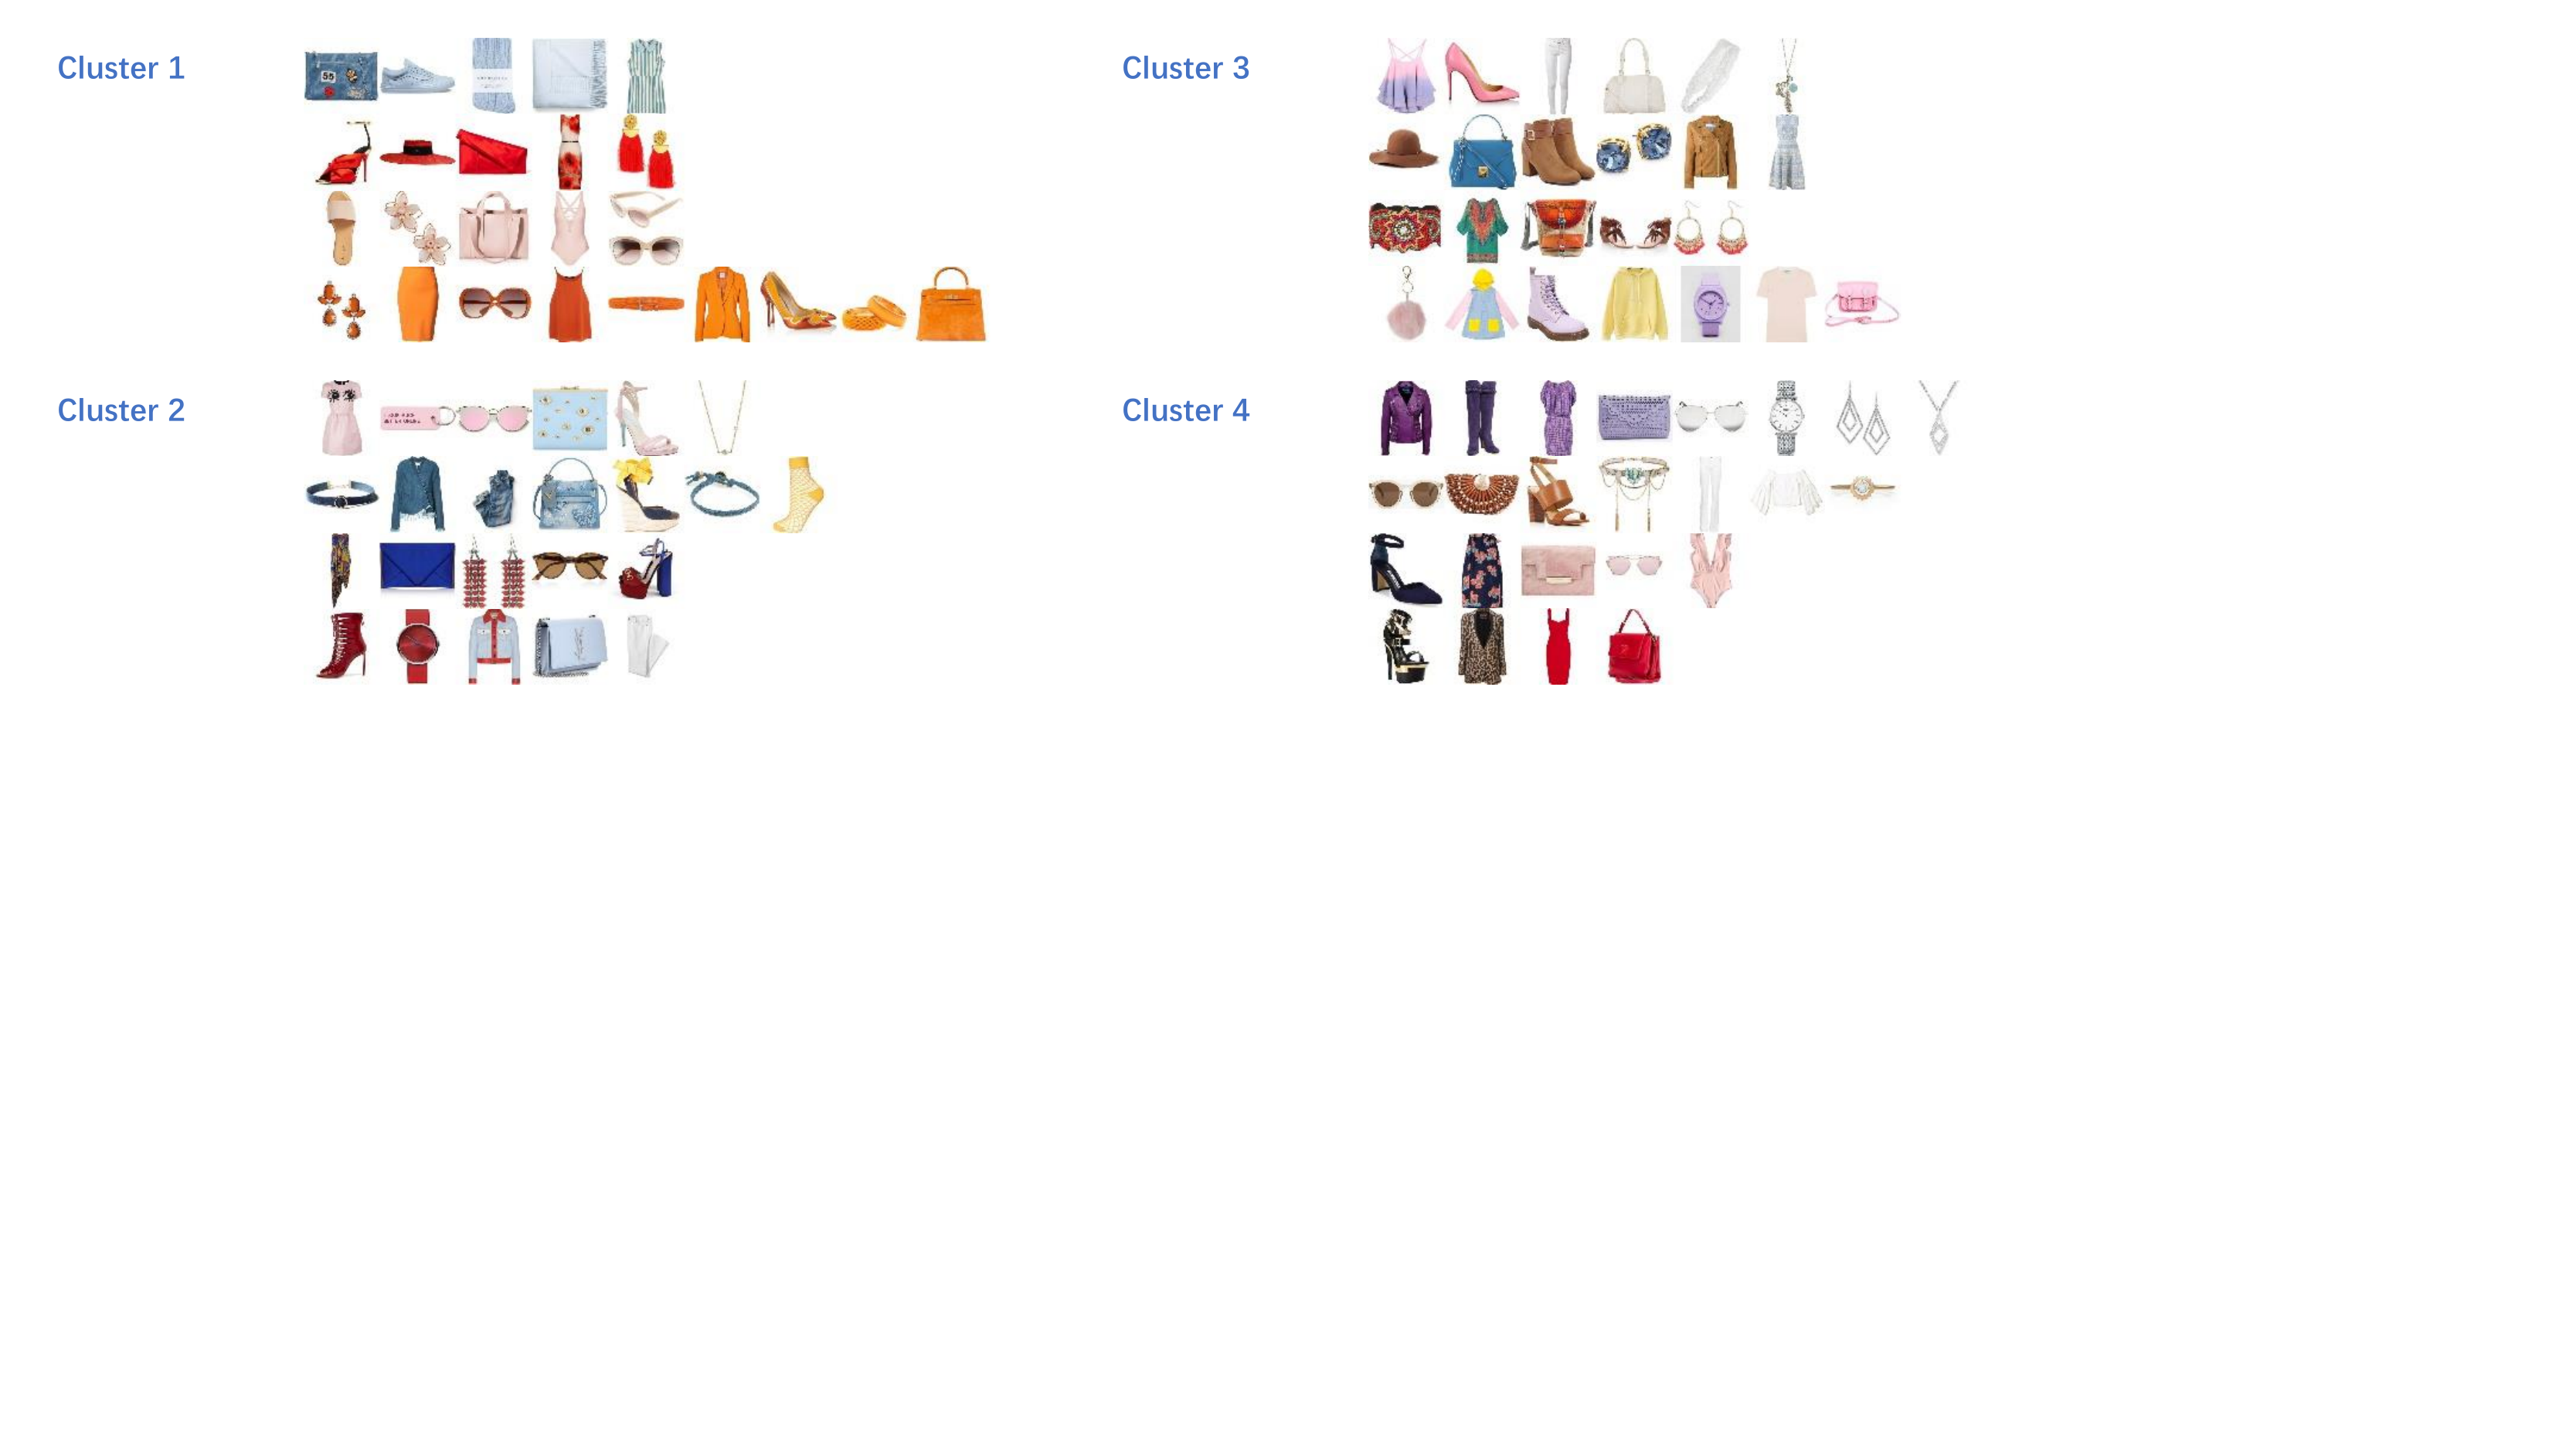}
\caption{Examples of outfits in each predicted cluster. The experiments were conducted on the testing set of the Polyvore Outfits dataset using the proposed method with color palettes. Each outfit is displayed in a row.}
\label{fig:supp_cluster}
\end{figure*}
