# Supplementary material for: Learning Color Compatibility in Fashion Outfits
Source: arXiv:2007.02388 source file (2020-07-05)
Supplement: Supplementary file 3 [file figure_supp_sample_it.tex]

\begin{figure*}
\begin{center}
\begin{subfigure}[b]{\linewidth}
	\centering
	\includegraphics[trim=0 0 0 0, clip,width=\linewidth]{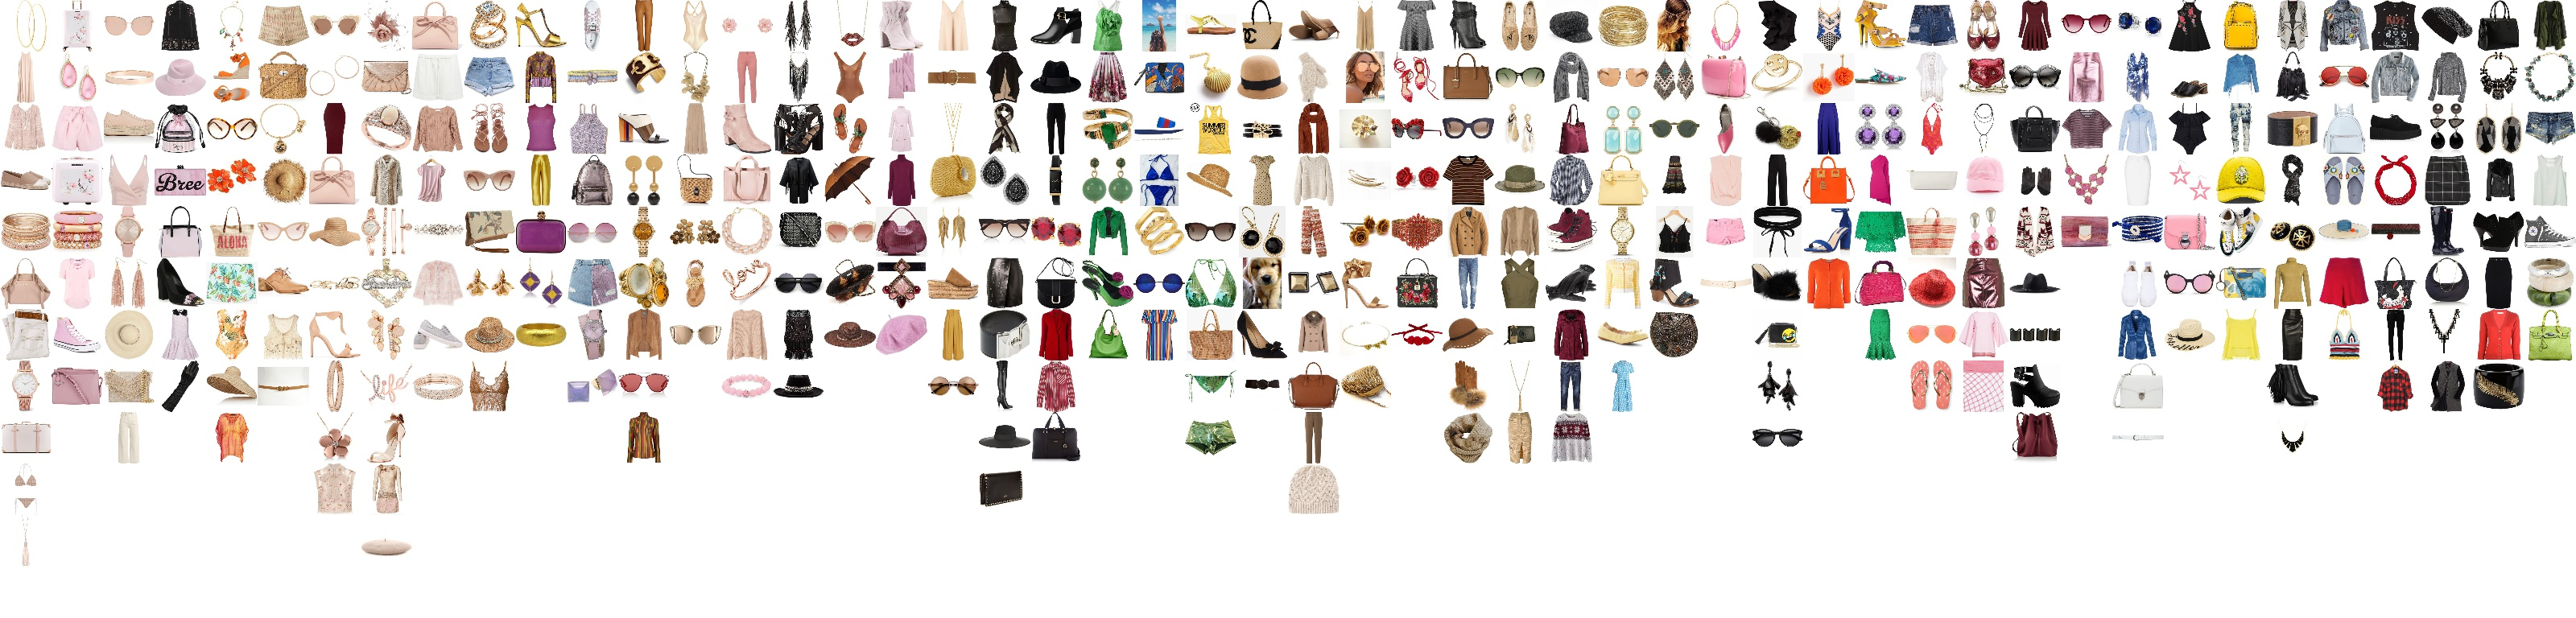}
	\caption{This cluster reveals two mixed color patterns. One pattern consists of similar colors, whereas the other pattern shows contrast colors.}
	\label{fig:supp_sample_it1}
\end{subfigure}
\begin{subfigure}[b]{\linewidth}
	\centering
	\includegraphics[trim=0 0 0 0, clip,width=\linewidth]{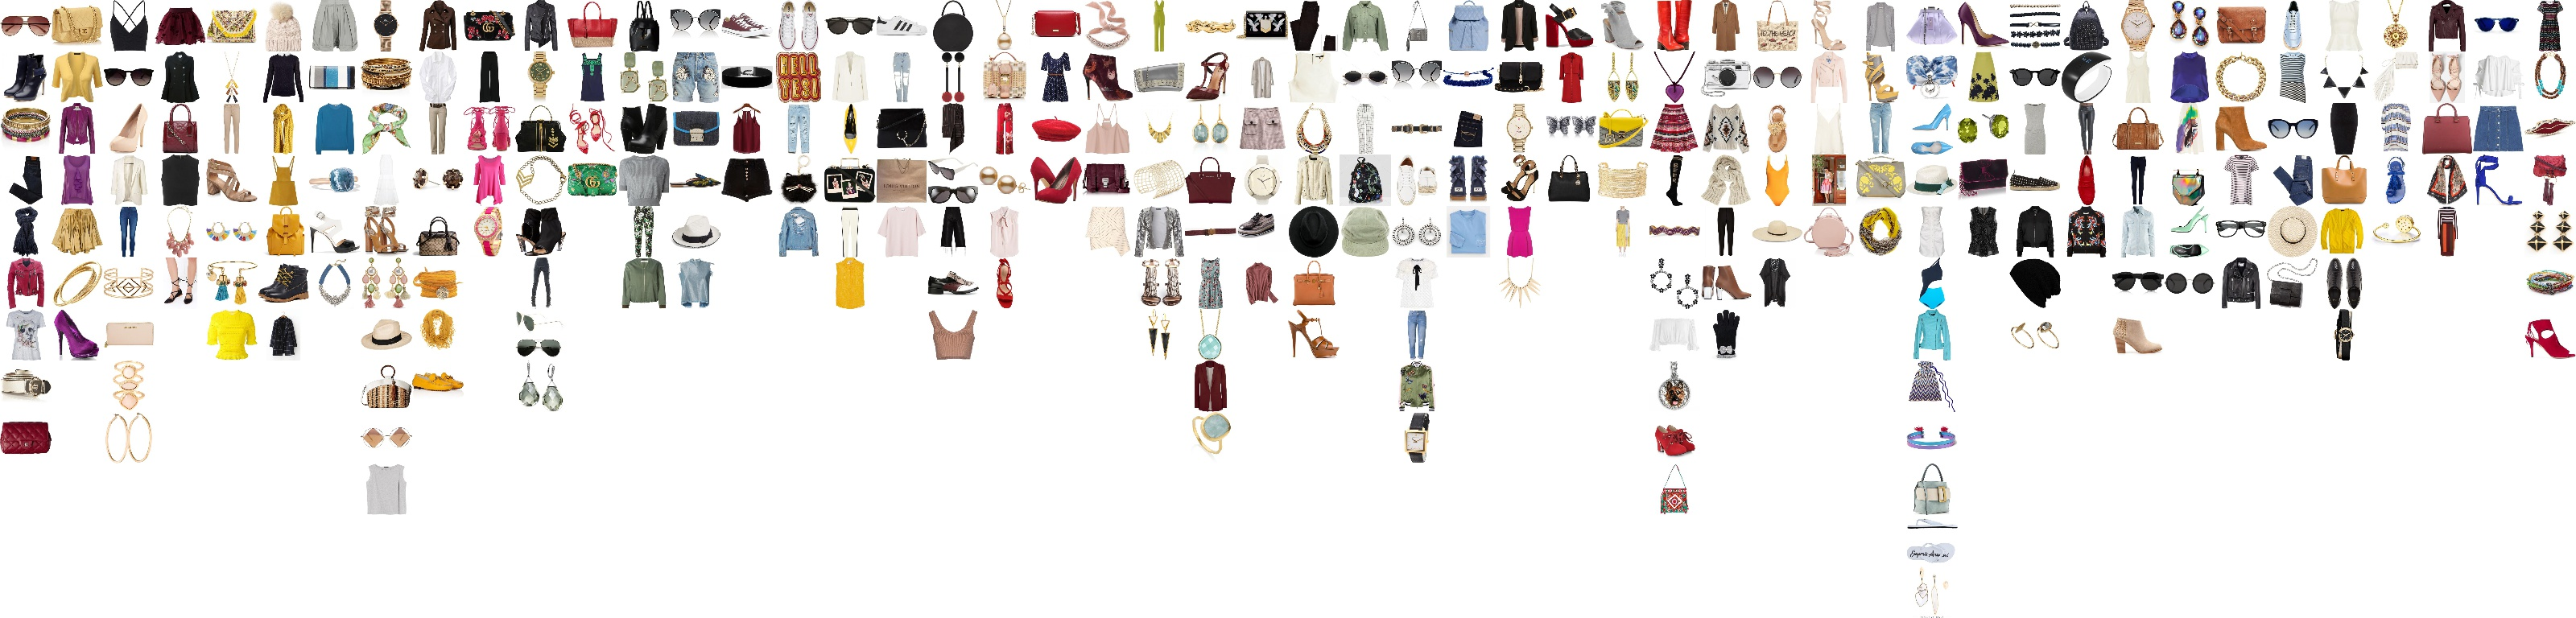}
	\caption{This cluster contains multiple color patterns that are hard to interpret directly.}
	\label{fig:supp_sample_it2}
\end{subfigure}
\end{center}
   \caption{Compatible outfit clusters predicted using color palettes as fashion representation. Due to limited space, we only display 50 outfits per cluster. The 50 outfits are shown on the left where items in the same column belong to the same outfit.}
\label{fig:supp_sample_it}
\end{figure*}
